# Supplementary material for: On the Effective Horizon of Inverse Reinforcement Learning
Source: arXiv:2307.06541 source file (2025-02-20)
Supplement: Supplementary file 1 [file cross_validation.tex]

\section{Detailed Results for Cross-Validation}

\begin{table*}[h]
    \centering
    \begin{tabular}{c}
\hspace{-5mm}
\includegraphics[width=1.05\textwidth]{fig/lp/gridworld/Gridworld-Simple_cross.jpg}
         \\ \hspace{-5mm}
         
      \includegraphics[width=1.05\textwidth]{fig/lp/gridworld/Gridworld-Hard_cross.jpg}
        \\ \hspace{-5mm}
        
        \includegraphics[width=1.05\textwidth]{fig/lp/objectworld/Objectworld-Linear_cross.jpg}
        \\ \hspace{-5mm}
        
        \includegraphics[width=1.05\textwidth]{fig/lp/objectworld/Objectworld-Non-linear_cross.jpg}
    \end{tabular}
    \caption{Using cross-validation to select $( \optimalR, \optimalGamma )$. The green curves are the ground truth error counts and the blue are for the validation error. The red markers highlight the top 10 best $\learnedGamma$s based on the ground-truth errors, while the orange markers highlights that based on the validation error. We only have access to the validation error curves when selecting $\optimalGamma$. 
    }
    \label{fig:cross_validate}
    \Description{CV}
\end{table*}
